# Supplementary material for: Bringing Light Into the Dark: A Large-scale Evaluation of Knowledge Graph Embedding Models Under a Unified Framework
Source: arXiv:2006.13365 source file (2021-11-01)
Supplement: Supplementary file 1 [file appendix_reproduction.tex]

%% ------FB15K
%% Average Ranking
\begin{table*}
\caption{Reproduction Results on FB15K Based On An Optimistic Ranking}
\label{tab:fb15k_full_results_average_ranking}
\centering
\begin{tabular}{lrrrrrrr}
\toprule
{} &               MR &           MRR (\%) &            AMR (\%) &        Hits@1 (\%) &        Hits@3 (\%) &        Hits@5 (\%) &     Hits@10 (\%) \\
\midrule
\textbf{ComplEx} &   171.16 $\pm$ 16.05 &  19.13 $\pm$ 0.45 &    2.46 $\pm$ 0.28 &  10.06 $\pm$ 0.42 &  20.82 $\pm$ 0.67 &  27.59 $\pm$ 0.94 &  38.03 $\pm$ 1.02 \\
\textbf{ConvE} &     50.76 $\pm$ 0.40 &  59.56 $\pm$ 0.06 &    0.73 $\pm$ 0.01 &  48.28 $\pm$ 0.12 &  66.99 $\pm$ 0.04 &  73.27 $\pm$ 0.03 &  79.76 $\pm$ 0.07 \\
\textbf{DistMult} &    134.02 $\pm$ 1.98 &  26.06 $\pm$ 0.17 &    1.86 $\pm$ 0.03 & 16.45 $\pm$ 0.16 &  29.10 $\pm$ 0.17 &  35.54 $\pm$ 0.21 &  45.00 $\pm$ 0.25 \\
\textbf{HolE} &    193.03 $\pm$ 7.61 &  34.15 $\pm$ 0.22 &    2.71 $\pm$ 0.12 &  21.79 $\pm$ 0.19 &  39.69 $\pm$ 0.24 &  48.06 $\pm$ 0.30 &  58.84 $\pm$ 0.28 \\
\textbf{KG2E} &  5779.07 $\pm$ 51.02 &   0.58 $\pm$ 0.07 &   78.40 $\pm$ 0.68 &   0.11 $\pm$ 0.04 &   0.36 $\pm$ 0.08 &   0.56 $\pm$ 0.10 &   1.01 $\pm$ 0.14 \\
\textbf{RotatE} &     42.28 $\pm$ 0.13 &  55.00 $\pm$ 0.06 &    0.63 $\pm$ 0.00 &  41.53 $\pm$ 0.06 &  64.14 $\pm$ 0.07 &  71.23 $\pm$ 0.05 &  78.67 $\pm$ 0.08 \\
\textbf{SimplE} &   7395.75 $\pm$ 2.02 &   0.04 $\pm$ 0.00 &  100.02 $\pm$ 0.03 &   0.01 $\pm$ 0.00 &   0.03 $\pm$ 0.00 &   0.04 $\pm$ 0.00 &   0.06 $\pm$ 0.01 \\
\textbf{TransD} &    153.37 $\pm$ 5.35 &  33.99 $\pm$ 0.03 &    2.29 $\pm$ 0.09 &  21.22 $\pm$ 0.03 &  40.48 $\pm$ 0.10 &  48.57 $\pm$ 0.09 &  58.71 $\pm$ 0.14 \\
\textbf{TransE} &    127.92 $\pm$ 0.86 &  26.01 $\pm$ 0.17 &    1.78 $\pm$ 0.01 &  15.23 $\pm$ 0.16 &  29.85 $\pm$ 0.24 &  37.18 $\pm$ 0.24 &  47.34 $\pm$ 0.18 \\
\textbf{TransH} &  6320.02 $\pm$ 30.37 &   2.54 $\pm$ 0.20 &   85.63 $\pm$ 0.40 &   1.69 $\pm$ 0.25 &   2.95 $\pm$ 0.20 &   3.29 $\pm$ 0.22 &   3.74 $\pm$ 0.18 \\
\textbf{TransR} &  6795.95 $\pm$ 16.65 &   0.65 $\pm$ 0.02 &   91.99 $\pm$ 0.22 &   0.37 $\pm$ 0.00 &   0.63 $\pm$ 0.04 &   0.78 $\pm$ 0.06 &   1.03 $\pm$ 0.07 \\
\textbf{TuckER} &  7327.77 $\pm$ 29.22 &   0.07 $\pm$ 0.02 &   99.11 $\pm$ 0.39 &   0.01 $\pm$ 0.00 &   0.02 $\pm$ 0.00 &   0.03 $\pm$ 0.01 &   0.15 $\pm$ 0.17 \\
\bottomrule
\end{tabular}
\end{table*}

%% Best Ranking
\begin{table*}
\caption{Reproduction Results on FB15K Based On An Optimistic Ranking}
\label{tab:fb15k_full_results_best_ranking}
\centering
\begin{tabular}{lrrrrrr}
\toprule
{} &               MR &           MRR (\%) &                Hits@1 (\%) &        Hits@3 (\%) &        Hits@5 (\%) &     Hits@10 (\%) \\
\midrule
\textbf{ComplEx} &   171.16 $\pm$ 16.05 &  19.13 $\pm$ 0.45 &  10.06 $\pm$ 0.42 &   20.82 $\pm$ 0.67 &   27.59 $\pm$ 0.94 &   38.03 $\pm$ 1.02 \\
\textbf{ConvE} &     50.76 $\pm$ 0.40 &  59.56 $\pm$ 0.06 &  48.28 $\pm$ 0.12 &   66.99 $\pm$ 0.04 &   73.27 $\pm$ 0.03 &   79.76 $\pm$ 0.07 \\
\textbf{DistMult} &    134.02 $\pm$ 1.98 &  26.06 $\pm$ 0.17 & 16.45 $\pm$ 0.16 &   29.10 $\pm$ 0.17 &   35.54 $\pm$ 0.21 &   45.00 $\pm$ 0.25 \\
\textbf{Hole} &    193.03 $\pm$ 7.61 &  34.15 $\pm$ 0.22 & 21.79 $\pm$ 0.19 &   39.69 $\pm$ 0.24 &   48.06 $\pm$ 0.30 &   58.84 $\pm$ 0.28 \\
\textbf{KG2E} &  5779.07 $\pm$ 51.02 &   0.58 $\pm$ 0.07 & 0.11 $\pm$ 0.04 &    0.36 $\pm$ 0.08 &    0.56 $\pm$ 0.10 &    1.01 $\pm$ 0.14 \\
\textbf{RotatE} &     42.28 $\pm$ 0.13 &  55.00 $\pm$ 0.06 & 41.53 $\pm$ 0.06 &   64.14 $\pm$ 0.07 &   71.23 $\pm$ 0.05 &   78.67 $\pm$ 0.08 \\
\textbf{SimplE} &   139.34 $\pm$ 49.45 &  23.90 $\pm$ 8.79 & 11.58 $\pm$ 6.42 &  24.16 $\pm$ 10.95 &  34.73 $\pm$ 13.40 &  54.28 $\pm$ 15.80 \\
\textbf{TransD} &    153.37 $\pm$ 5.35 &  33.99 $\pm$ 0.03 & 21.22 $\pm$ 0.03 &   40.48 $\pm$ 0.10 &   48.57 $\pm$ 0.09 &   58.71 $\pm$ 0.14 \\
\textbf{TransE} &    127.92 $\pm$ 0.86 &  26.01 $\pm$ 0.17 & 15.23 $\pm$ 0.16 &   29.85 $\pm$ 0.24 &   37.18 $\pm$ 0.24 &   47.34 $\pm$ 0.18 \\
\textbf{TransH} &  6320.00 $\pm$ 30.37 &   2.54 $\pm$ 0.20 & 1.69 $\pm$ 0.25 &    2.95 $\pm$ 0.20 &    3.29 $\pm$ 0.22 &    3.74 $\pm$ 0.18 \\
\textbf{TransR} &  6795.94 $\pm$ 16.65 &   0.65 $\pm$ 0.02 & 0.37 $\pm$ 0.00 &    0.63 $\pm$ 0.04 &    0.78 $\pm$ 0.06 &    1.03 $\pm$ 0.07 \\
\textbf{TuckER} &  7327.77 $\pm$ 29.22 &   0.07 $\pm$ 0.02 &   0.01 $\pm$ 0.00 &    0.02 $\pm$ 0.00 &    0.03 $\pm$ 0.01 &    0.15 $\pm$ 0.17 \\
\bottomrule
\end{tabular}
\end{table*}

%% Worst Ranking
\begin{table*}
\caption{Reproduction Results on FB15K Based On A Pessimistic Ranking}
\label{tab:fb15k_full_results_worst_ranking}
\centering
\begin{tabular}{lrrrrrr}
\toprule
{} &               MR &           MRR (\%) &                Hits@1 (\%) &        Hits@3 (\%) &        Hits@5 (\%) &     Hits@10 (\%) \\
\midrule
\textbf{ComplEx} &    171.16 $\pm$ 16.05 &  19.13 $\pm$ 0.45 &  10.06 $\pm$ 0.42 &  20.82 $\pm$ 0.67 &  27.59 $\pm$ 0.94 &  38.03 $\pm$ 1.02 \\
\textbf{ConvE} &      50.76 $\pm$ 0.40 &  59.56 $\pm$ 0.06 &  48.28 $\pm$ 0.12 &  66.99 $\pm$ 0.04 &  73.27 $\pm$ 0.03 &  79.76 $\pm$ 0.07 \\
\textbf{DistMult} &     134.02 $\pm$ 1.98 &  26.06 $\pm$ 0.17 &  16.45 $\pm$ 0.16 &  29.10 $\pm$ 0.17 &  35.54 $\pm$ 0.21 &  45.00 $\pm$ 0.25 \\
\textbf{HolE} &     193.03 $\pm$ 7.61 &  34.15 $\pm$ 0.22 &  21.79 $\pm$ 0.19 &  39.69 $\pm$ 0.24 &  48.06 $\pm$ 0.30 &  58.84 $\pm$ 0.28 \\
\textbf{KG2E} &   5779.07 $\pm$ 51.02 &   0.58 $\pm$ 0.07 &   0.11 $\pm$ 0.04 &   0.36 $\pm$ 0.08 &   0.56 $\pm$ 0.10 &   1.01 $\pm$ 0.14 \\
\textbf{RotatE} &      42.28 $\pm$ 0.13 &  55.00 $\pm$ 0.06 &  41.53 $\pm$ 0.06 &  64.14 $\pm$ 0.07 &  71.23 $\pm$ 0.05 &  78.67 $\pm$ 0.08 \\
\textbf{SimplE} &  14652.16 $\pm$ 45.71 &   0.03 $\pm$ 0.00 &   0.01 $\pm$ 0.00 &   0.03 $\pm$ 0.00 &   0.04 $\pm$ 0.00 &   0.06 $\pm$ 0.01 \\
\textbf{TransD} &     153.37 $\pm$ 5.35 &  33.99 $\pm$ 0.03 &  21.22 $\pm$ 0.03 &  40.48 $\pm$ 0.10 &  48.57 $\pm$ 0.09 &  58.71 $\pm$ 0.14 \\
\textbf{TransE} &     127.92 $\pm$ 0.86 &  26.01 $\pm$ 0.17 &  15.23 $\pm$ 0.16 &  29.85 $\pm$ 0.24 &  37.18 $\pm$ 0.24 &  47.34 $\pm$ 0.18 \\
\textbf{TransH} &   6320.05 $\pm$ 30.37 &   2.54 $\pm$ 0.20 &   1.69 $\pm$ 0.25 &   2.95 $\pm$ 0.20 &   3.29 $\pm$ 0.22 &   3.74 $\pm$ 0.18 \\
\textbf{TransR} &   6795.95 $\pm$ 16.65 &   0.65 $\pm$ 0.02 &   0.37 $\pm$ 0.00 &   0.63 $\pm$ 0.04 &   0.78 $\pm$ 0.06 &   1.03 $\pm$ 0.07 \\
\textbf{TuckER} &   7327.77 $\pm$ 29.22 &   0.07 $\pm$ 0.02 &   0.01 $\pm$ 0.00 &   0.02 $\pm$ 0.00 &   0.03 $\pm$ 0.01 &   0.15 $\pm$ 0.17 \\
\bottomrule
\end{tabular}
\end{table*}

% --------WN18--------
%

\begin{table*}
\caption{Reproduction Results on WN18 Based On An Average Ranking}
\label{tab:wn18_full_results_average_ranking}
\centering
\begin{tabular}{lrrrrrrr}
\toprule
{} &               MR &           MRR (\%) &            AMR (\%) &        Hits@1 (\%) &        Hits@3 (\%) &        Hits@5 (\%) &     Hits@10 (\%) \\
\midrule
\textbf{ComplEx} &     452.67 $\pm$ 63.05 &  19.49 $\pm$ 2.55 &    2.21 $\pm$ 0.31 &  12.36 $\pm$ 1.96 &  20.66 $\pm$ 2.75 &  25.24 $\pm$ 3.33 &  32.92 $\pm$ 4.40 \\
\textbf{ConvE} &     444.40 $\pm$ 14.82 &  88.81 $\pm$ 0.09 &    2.17 $\pm$ 0.07 &  85.14 $\pm$ 0.10 &  91.76 $\pm$ 0.11 &  93.29 $\pm$ 0.04 &  94.85 $\pm$ 0.06 \\
\textbf{DistMult} &     458.64 $\pm$ 23.96 &  77.44 $\pm$ 0.22 &    2.24 $\pm$ 0.12 &  67.45 $\pm$ 0.34 &  85.94 $\pm$ 0.21 &  89.52 $\pm$ 0.25 &  92.72 $\pm$ 0.18 \\
\textbf{HolE} &     812.64 $\pm$ 28.33 &  70.44 $\pm$ 0.45 &    3.97 $\pm$ 0.14 &  59.29 $\pm$ 0.53 &  79.29 $\pm$ 0.47 &  84.12 $\pm$ 0.36 &  88.61 $\pm$ 0.42 \\
\textbf{KG2E} &    2708.89 $\pm$ 44.57 &   3.61 $\pm$ 0.26 &   13.25 $\pm$ 0.22 &   1.35 $\pm$ 0.22 &   3.21 $\pm$ 0.31 &   4.57 $\pm$ 0.34 &   7.02 $\pm$ 0.43 \\
\textbf{RotatE} &      123.68 $\pm$ 1.71 &  87.29 $\pm$ 0.12 &    0.61 $\pm$ 0.01 &  82.17 $\pm$ 0.20 &  91.53 $\pm$ 0.12 &  93.44 $\pm$ 0.07 &  95.28 $\pm$ 0.08 \\
\textbf{SimplE} &   20376.43 $\pm$ 42.30 &   0.04 $\pm$ 0.01 &   99.57 $\pm$ 0.21 &   0.01 $\pm$ 0.01 &   0.03 $\pm$ 0.00 &   0.04 $\pm$ 0.01 &   0.07 $\pm$ 0.03 \\
\textbf{TransD} &     444.39 $\pm$ 25.61 &  36.22 $\pm$ 0.12 &    2.17 $\pm$ 0.13 &   3.94 $\pm$ 0.27 &  65.63 $\pm$ 0.55 &  79.64 $\pm$ 0.43 &  87.27 $\pm$ 0.41 \\
\textbf{TransE} &     468.24 $\pm$ 13.64 &  39.19 $\pm$ 1.21 &    2.29 $\pm$ 0.07 &   9.99 $\pm$ 1.82 &  64.74 $\pm$ 0.91 &  75.44 $\pm$ 0.48 &  84.25 $\pm$ 0.33 \\
\textbf{TransH} &   19678.04 $\pm$ 18.92 &   0.18 $\pm$ 0.04 &   96.16 $\pm$ 0.09 &   0.04 $\pm$ 0.02 &  0.19 $\pm$ 0.10 &   0.29 $\pm$ 0.14 &   0.39 $\pm$ 0.11 \\
\textbf{TransR} &  19686.49 $\pm$ 100.97 &   0.06 $\pm$ 0.02 &   96.20 $\pm$ 0.49 &   0.00 $\pm$ 0.00 &   0.04 $\pm$ 0.02 &   0.05 $\pm$ 0.03 &   0.11 $\pm$ 0.06 \\
\textbf{TuckER} &  20622.46 $\pm$ 153.52 &   0.03 $\pm$ 0.01 &  100.78 $\pm$ 0.75 &   0.00 $\pm$ 0.00 &   0.02 $\pm$ 0.01 &   0.03 $\pm$ 0.03 &   0.04 $\pm$ 0.03 \\
\bottomrule
\end{tabular}
\end{table*}

% WN18 Optimistic Ranking
\begin{table*}
\caption{Reproduction Results on WN18 Based On An Optimistic Ranking}
\label{tab:wn18_full_results_optimistic_ranking}
\centering
\begin{tabular}{lrrrrrrr}
\toprule
{} &               MR &           MRR (\%) &           Hits@1 (\%) &        Hits@3 (\%) &        Hits@5 (\%) &     Hits@10 (\%) \\
\midrule
\textbf{ComplEx} &     452.67 $\pm$ 63.05 &  19.49 $\pm$ 2.55 &  12.36 $\pm$ 1.96 &  20.66 $\pm$ 2.75 &  25.24 $\pm$ 3.33 &  32.92 $\pm$ 4.40 \\
\textbf{ConvE} &     444.40 $\pm$ 14.82 &  88.81 $\pm$ 0.09 &  85.14 $\pm$ 0.10 &  91.76 $\pm$ 0.11 &  93.29 $\pm$ 0.04 &  94.85 $\pm$ 0.06 \\
\textbf{DistmMlt} &     458.64 $\pm$ 23.96 &  77.44 $\pm$ 0.22 &  67.45 $\pm$ 0.34 &  85.94 $\pm$ 0.21 &  89.52 $\pm$ 0.25 &  92.72 $\pm$ 0.18 \\
\textbf{HolE} &     812.63 $\pm$ 28.33 &  70.44 $\pm$ 0.45 &  59.29 $\pm$ 0.53 &  79.29 $\pm$ 0.47 &  84.12 $\pm$ 0.36 &  88.61 $\pm$ 0.42 \\
\textbf{KG2E} &    2708.88 $\pm$ 44.57 &   3.61 $\pm$ 0.26 &   1.35 $\pm$ 0.22 &   3.21 $\pm$ 0.31 &   4.57 $\pm$ 0.34 &   7.02 $\pm$ 0.43 \\
\textbf{RotatE} &      123.68 $\pm$ 1.71 &  87.29 $\pm$ 0.12 &  82.17 $\pm$ 0.20 &  91.53 $\pm$ 0.12 &  93.44 $\pm$ 0.07 &  95.28 $\pm$ 0.08 \\
\textbf{SimplE} &     384.53 $\pm$ 66.45 &  38.48 $\pm$ 4.00 &  33.93 $\pm$ 4.32 &  39.59 $\pm$ 4.67 &  42.76 $\pm$ 3.73 &  47.01 $\pm$ 2.66 \\
\textbf{TransD} &     444.39 $\pm$ 25.61 &  36.22 $\pm$ 0.12  &  3.94 $\pm$ 0.27 &  65.63 $\pm$ 0.55 &  79.64 $\pm$ 0.43 &  87.27 $\pm$ 0.41 \\
\textbf{TransE } &     468.24 $\pm$ 13.64 &  39.19 $\pm$ 1.21 &   9.99 $\pm$ 1.82 &  64.74 $\pm$ 0.91 &  75.44 $\pm$ 0.48 &  84.25 $\pm$ 0.33 \\
\textbf{TransH} &   19678.02 $\pm$ 18.92 &   0.18 $\pm$ 0.04 &   0.04 $\pm$ 0.02 &   0.19 $\pm$ 0.10 &   0.29 $\pm$ 0.14 &   0.39 $\pm$ 0.11 \\
\textbf{TransR} &  19686.49 $\pm$ 100.97 &   0.06 $\pm$ 0.02 &   0.00 $\pm$ 0.00 &   0.04 $\pm$ 0.02 &   0.05 $\pm$ 0.03 &   0.11 $\pm$ 0.06 \\
\textbf{TuckER} &  20622.46 $\pm$ 153.52 &   0.03 $\pm$ 0.01 &   0.00 $\pm$ 0.00 &   0.02 $\pm$ 0.01 &   0.03 $\pm$ 0.03 &   0.04 $\pm$ 0.03 \\
\bottomrule
\end{tabular}
\end{table*}

% WN18 Worst Ranking
\begin{table*}
\caption{Reproduction Results on WN18 Based On A Pessimistic Ranking}
\label{tab:wn18_full_results_pessimistic_ranking}
\centering
\begin{tabular}{lrrrrrrr}
\toprule
{} &               MR &           MRR (\%) &           Hits@1 (\%) &        Hits@3 (\%) &        Hits@5 (\%) &     Hits@10 (\%) \\
\midrule
\textbf{ComplEx} &     452.67 $\pm$ 63.05 &  19.49 $\pm$ 2.55 &  12.36 $\pm$ 1.96 &  20.66 $\pm$ 2.75 &  25.24 $\pm$ 3.33 &  32.92 $\pm$ 4.40 \\
\textbf{ConvE} &     444.40 $\pm$ 14.82 &  88.81 $\pm$ 0.09 &  85.14 $\pm$ 0.10 &  91.76 $\pm$ 0.11 &  93.29 $\pm$ 0.04 &  94.85 $\pm$ 0.06 \\
\textbf{DistMult} &     458.64 $\pm$ 23.96 &  77.44 $\pm$ 0.22 &  67.45 $\pm$ 0.34 &  85.94 $\pm$ 0.21 &  89.52 $\pm$ 0.25 &  92.72 $\pm$ 0.18 \\
\textbf{HolE} &     812.64 $\pm$ 28.34 &  70.44 $\pm$ 0.45 &  59.29 $\pm$ 0.53 &  79.29 $\pm$ 0.47 &  84.12 $\pm$ 0.36 &  88.61 $\pm$ 0.42 \\
\textbf{KG2E} &    2708.89 $\pm$ 44.57 &   3.61 $\pm$ 0.26 &   1.35 $\pm$ 0.22 &   3.21 $\pm$ 0.31 &   4.57 $\pm$ 0.34 &   7.02 $\pm$ 0.43 \\
\textbf{RotatE} &      123.68 $\pm$ 1.71 &  87.29 $\pm$ 0.12  &  82.17 $\pm$ 0.20 &  91.53 $\pm$ 0.12 &  93.44 $\pm$ 0.07 &  95.28 $\pm$ 0.08 \\
\textbf{SimplE} &  40368.33 $\pm$ 114.95 &   0.03 $\pm$ 0.01 &   0.01 $\pm$ 0.01 &   0.03 $\pm$ 0.00 &   0.04 $\pm$ 0.01 &   0.07 $\pm$ 0.03 \\
\textbf{TransD} &     444.39 $\pm$ 25.61 &  36.22 $\pm$ 0.12 &   3.94 $\pm$ 0.27 &  65.63 $\pm$ 0.55 &  79.64 $\pm$ 0.43 &  87.27 $\pm$ 0.41 \\
\textbf{TransE} &     468.24 $\pm$ 13.64 &  39.19 $\pm$ 1.21 &   9.99 $\pm$ 1.82 &  64.74 $\pm$ 0.91 &  75.44 $\pm$ 0.48 &  84.25 $\pm$ 0.33 \\
\textbf{TransH} &   19678.06 $\pm$ 18.92 &   0.18 $\pm$ 0.04 &   0.04 $\pm$ 0.02 &   0.19 $\pm$ 0.10 &   0.29 $\pm$ 0.14 &   0.39 $\pm$ 0.11 \\
\textbf{TransR} &  19686.50 $\pm$ 100.97 &   0.06 $\pm$ 0.02 &   0.00 $\pm$ 0.00 &   0.04 $\pm$ 0.02 &   0.05 $\pm$ 0.03 &   0.11 $\pm$ 0.06 \\
\textbf{TuckER} &  20622.46 $\pm$ 153.52 &   0.03 $\pm$ 0.01 &   0.00 $\pm$ 0.00 &   0.02 $\pm$ 0.01 &   0.03 $\pm$ 0.03 &   0.04 $\pm$ 0.03 \\
\bottomrule
\end{tabular}
\end{table*}

%
% --------FB15K-237--------
%

\begin{table*}[t]
\caption{Reproduction Results on FB15K-237 Based On An Average Ranking}
\label{fb15k237_full_results_average_ranking}
\centering
\begin{tabular}{lrrrrrrr}
\toprule
{} &               MR &           MRR (\%) &            AMR (\%) &        Hits@1 (\%) &        Hits@3 (\%) &        Hits@5 (\%) &     Hits@10 (\%) \\
\midrule

\textbf{ConvE} &  255.46 $\pm$ 6.16 &  26.93 $\pm$ 0.11 &  3.73 $\pm$ 0.13 &  18.22 $\pm$ 0.11 &  29.51 $\pm$ 0.24 &  35.98 $\pm$ 0.16 &  44.95 $\pm$ 0.17 \\
\textbf{ConvKB} &  4345.27 $\pm$ 46.99 &   4.71 $\pm$ 0.23 &  61.36 $\pm$ 0.65 &   3.31 $\pm$ 0.23 &   4.04 $\pm$ 0.19 &   4.57 $\pm$ 0.22 &   7.76 $\pm$ 0.88 \\
\textbf{RotatE} &  191.92 $\pm$ 0.31 &  26.42 $\pm$ 0.04 &  2.84 $\pm$ 0.00 &  17.57 $\pm$ 0.06 &  28.97 $\pm$ 0.05 &  35.29 $\pm$ 0.09 &  44.55 $\pm$ 0.06 \\

\bottomrule
\end{tabular}
\end{table*}

\begin{table*}[t]
\caption{Reproduction Results on FB15K-237 Based On An Optimistic Ranking}
\label{fb15k237_full_results_optimistic_ranking}
\centering
\begin{tabular}{lrrrrrr}
\toprule
{} &               MR &           MRR (\%) &              Hits@1 (\%) &        Hits@3 (\%) &        Hits@5 (\%) &     Hits@10 (\%) \\
\midrule

\textbf{ConvE} &  255.46 $\pm$ 6.16 &  26.93 $\pm$ 0.11 &  18.22 $\pm$ 0.11 &  29.51 $\pm$ 0.24 &  35.98 $\pm$ 0.16 &  44.95 $\pm$ 0.17 \\
\textbf{ConvKB} &  4345.27 $\pm$ 46.99 &   4.71 $\pm$ 0.23 &  3.31 $\pm$ 0.23 &   4.04 $\pm$ 0.19 &   4.57 $\pm$ 0.22 &   7.76 $\pm$ 0.88 \\
\textbf{RotatE} &  191.92 $\pm$ 0.31 &  26.42 $\pm$ 0.04 &  17.57 $\pm$ 0.06 &  28.97 $\pm$ 0.05 &  35.29 $\pm$ 0.09 &  44.55 $\pm$ 0.06 \\

\bottomrule
\end{tabular}
\end{table*}

\begin{table*}[t]
\caption{Reproduction Results on FB15K-237 Based On A Pessimistic Ranking}
\label{fb15k237_full_results_pessimistic_ranking}
\centering
\begin{tabular}{lrrrrrr}
\toprule
{} &               MR &           MRR (\%) &              Hits@1 (\%) &        Hits@3 (\%) &        Hits@5 (\%) &     Hits@10 (\%) \\
\midrule

\textbf{ConvE} &  255.46 $\pm$ 6.16 &  26.93 $\pm$ 0.11 &  18.22 $\pm$ 0.11 &  29.51 $\pm$ 0.24 &  35.98 $\pm$ 0.16 &  44.95 $\pm$ 0.17 \\
\textbf{ConvKB} &  4345.27 $\pm$ 46.99 &   4.71 $\pm$ 0.23 &   3.31 $\pm$ 0.23 &   4.04 $\pm$ 0.19 &   4.57 $\pm$ 0.22 &   7.76 $\pm$ 0.88 \\
\textbf{RotatE} &  191.92 $\pm$ 0.31 &  26.42 $\pm$ 0.04 &  17.57 $\pm$ 0.06 &  28.97 $\pm$ 0.05 &  35.29 $\pm$ 0.09 &  44.55 $\pm$ 0.06 \\
\bottomrule
\end{tabular}
\end{table*}

% --------WN18RR--------
%

\begin{table*}[t]
\caption{Reproduction Results on WN18RR Based On An Average Ranking}
\label{wn18rr_full_results_average_ranking}
\centering
\begin{tabular}{lrrrrrrr}
\toprule
{} &               MR &           MRR (\%) &            AMR (\%) &        Hits@1 (\%) &        Hits@3 (\%) &        Hits@5 (\%) &     Hits@10 (\%) \\
\midrule
\textbf{ConvE} &  5369.49 $\pm$ 50.92 &  44.69 $\pm$ 0.21 &  26.49 $\pm$ 0.25 &  40.98 $\pm$ 0.22 &  46.49 $\pm$ 0.14 &  48.92 $\pm$ 0.23 &  51.76 $\pm$ 0.13 \\
\textbf{ConvKB} &  13634.66 $\pm$ 714.24 &   0.30 $\pm$ 0.07 &  67.27 $\pm$ 3.52 &   0.09 $\pm$ 0.03 &   0.21 $\pm$ 0.07 &   0.32 $\pm$ 0.10 &   0.57 $\pm$ 0.16 \\
\textbf{RotatE} &  4263.32 $\pm$ 90.33 &  48.40 $\pm$ 0.09 &  21.03 $\pm$ 0.45 &  44.02 $\pm$ 0.15 &  50.55 $\pm$ 0.12 &  52.98 $\pm$ 0.11 &  56.51 $\pm$ 0.26 \\
\bottomrule
\end{tabular}
\end{table*}

\begin{table*}[t]
\caption{Reproduction Results on WN18RR Based On An Optimistic Ranking}
\label{wn18rr_full_results_optimistic_ranking}
\centering
\begin{tabular}{lrrrrrr}
\toprule
{} &               MR &           MRR (\%) &           Hits@1 (\%) &        Hits@3 (\%) &        Hits@5 (\%) &     Hits@10 (\%) \\
\midrule
\textbf{ConvE} &  5369.49 $\pm$ 50.92 &  44.69 $\pm$ 0.21 &  40.98 $\pm$ 0.22 &  46.49 $\pm$ 0.14 &  48.92 $\pm$ 0.23 &  51.76 $\pm$ 0.13 \\
\textbf{ConvKB} &  13634.65 $\pm$ 714.24 &   0.30 $\pm$ 0.07 &  0.09 $\pm$ 0.03 &   0.21 $\pm$ 0.07 &   0.32 $\pm$ 0.10 &   0.57 $\pm$ 0.16 \\
\textbf{RotatE} &  4263.32 $\pm$ 90.33 &  48.40 $\pm$ 0.09 &  44.02 $\pm$ 0.15 &  50.55 $\pm$ 0.12 &  52.98 $\pm$ 0.11 &  56.51 $\pm$ 0.26 \\
\bottomrule
\end{tabular}
\end{table*}

\begin{table*}[t]
\caption{Reproduction Results on WN18RR Based On A Pessimistic Ranking}
\label{wn18rr_full_results_pessimistic_ranking}
\centering
\begin{tabular}{lrrrrrr}
\toprule
{} &               MR &           MRR (\%) &           Hits@1 (\%) &        Hits@3 (\%) &        Hits@5 (\%) &     Hits@10 (\%) \\
\midrule
\textbf{ConvE} &  5369.49 $\pm$ 50.92 &  44.69 $\pm$ 0.21 &  40.98 $\pm$ 0.22 &  46.49 $\pm$ 0.14 &  48.92 $\pm$ 0.23 &  51.76 $\pm$ 0.13 \\
\textbf{ConvKB} &  13634.66 $\pm$ 714.24 &   0.30 $\pm$ 0.07 &   0.09 $\pm$ 0.03 &   0.21 $\pm$ 0.07 &   0.32 $\pm$ 0.10 &   0.57 $\pm$ 0.16 \\
\textbf{RotatE} &  4263.32 $\pm$ 90.33 &  48.40 $\pm$ 0.09 &  44.02 $\pm$ 0.15 &  50.55 $\pm$ 0.12 &  52.98 $\pm$ 0.11 &  56.51 $\pm$ 0.26 \\
\bottomrule
\end{tabular}
\end{table*}
